# Supplementary material for: Contrastive Learning for Enhancing Robust Scene Transfer in Vision-based Agile Flight
Source: arXiv:2309.09865 source file (2024-02-29)
Supplement: Supplementary file 1 [file supplementary_material.tex]

\section*{Supplementary Material}\label{sec:SupplementaryMaterial}
\textbf{Video: }\href{https://youtu.be/4A4YyPgEWD8}{https://youtu.be/4A4YyPgEWD8}
